# Supplementary material for: Simultaneous Broadband Vector Magnetometry Using Solid-State Spins
Source: arXiv:1803.03718 ancillary file (2018-03-26)
Supplement: Supplementary file 1 [file SM.pdf]

# Supplemental Material: Simultaneous Broadband Vector Magnetometry Using Solid-State Spins

Jennifer M. Schloss,[1,2] John F. Barry,[2,3,4,5] Matthew J. Turner,[2,5] and Ronald L. Walsworth[2,4,5]

[1]*Department of Physics, Massachusetts Institute of Technology, Cambridge, Massachusetts 02139, USA*
[2]*Center for Brain Science, Harvard University, Cambridge, Massachusetts 02138, USA*
[3]*Lincoln Laboratory, Massachusetts Institute of Technology, Lexington, Massachusetts 02420, USA*
[4]*Harvard-Smithsonian Center for Astrophysics, Cambridge, Massachusetts 02138, USA*
[5]*Department of Physics, Harvard University, Cambridge, Massachusetts 02138, USA*

(Dated: March 26, 2018)

## S1. BANDWIDTH AND SIGNAL-TO-NOISE RATIO

For a nitrogen-vacancy (NV) ensemble-based magnetometer that interrogates NV orientations sequentially, a measurement of the full vector magnetic field exhibits a reduced maximum bandwidth relative to a measurement of a single magnetic field component on the same device. The bandwidth difference arises because the full magnetic field vector must be deduced from multiple measurements interrogating different NV orientations. If a measurement using a single NV orientation requires time $T$, a sequential measurement utilizing all four NV orientations will require time $4T$ to sense the full vector magnetic field. Thus, the maximum bandwidth of a full vector magnetic field measurement utilizing all four NV orientations is $4\times$ lower than for a magnetic field measurement utilizing a single NV orientation.

In contrast, for a simultaneous vector magnetometry measurement, each NV orientation is interrogated for the full measurement time. Because the measurement signal-to-noise ratio (SNR) scales as $\sqrt{T}$ for statistically uncorrelated noise, the simultaneous technique achieves $2\times$ the SNR for each NV orientation as the sequential measurement. In practice, the relative SNR enhancement may be higher than $2\times$, as a sequential measurement using a single microwave (MW) generator may suffer from dead time when the MW carrier frequency is switched between the optically detected magnetic resonance (ODMR) features from different NV orientations.

## S2. MITIGATION OF CROSS-EXCITATION AND INTERMODULATION

Here we discuss cross-talk issues that may degrade the performance of a simultaneous vector magnetometer. First, off-resonant excitation of one NV orientation by MWs intended to drive another NV orientation is a general concern for both simultaneous and sequential vector magnetic field sensing as well as single-axis sensing from NV ensembles. This type of cross-talk is mitigated in this work by using a sufficiently strong bias magnetic field to spectrally separate the NV ODMR features. Modulated ODMR [1] is less sensitive to off-resonant excitation than conventional continuous-wave (CW) ODMR because the MW frequency modulation and subsequent lock-in detection generates a dispersion-type signal, which is approximately proportional to the derivative of the ODMR lineshape [2, 3]. In an NV ensemble, the ODMR features exhibit approximately Lorentzian lineshapes [4]; at large detunings $\Delta$ compared to the full width at half maximum $\Gamma$ of a Lorentzian-type feature ($\Delta \gg \Gamma$), the Lorentzian wings decay as $\sim 1/\Delta^2$. As a result, the change in detected PL in response to a small magnetic field deviation, i.e., $d\mathrm{PL}/dB_i(\Delta)$, falls off as $\sim 1/\Delta^3$. Meanwhile, the wings of the dispersion-type lock-in signal decay as $\sim 1/\Delta^3$ far off resonance. Therefore, response of the lock-in signal $S_i$ to a small magnetic field deviation, $dS_i/dB_i(\Delta)$, scales as $\sim 1/\Delta^4$. This $\sim 1/\Delta^4$ fall-off was confirmed experimentally by applying an 18 Hz magnetic field along the lab-frame $z$-axis and detecting the signal on the channel corresponding to the highest-frequency ODMR line, centered at $\nu_{\kappa^+}$ (see main text and Fig. 1(d)), using a MW drive with carrier frequency detuning varied from +5 MHz to +15 MHz. At the applied $\vec{B}_0$, the nearest two hyperfine ODMR subfeatures from different NV orientations are separated by 30 MHz, which is large compared to the $\sim$ MHz ODMR linewidths, so we conclude that off-resonant cross excitation during vector magnetometry measurements is negligible.

Second, if multiple MW tones $\nu_i$ pass through the same MW amplifier, the amplifier's nonlinear response near saturation may cause intermodulation. In particular, third-order products $2\nu_i - \nu_j$ may drive NV spin transitions if they happen to coincide with any of the ODMR features. The present device mitigates this effect by using four MW amplifiers, one for each MW carrier frequency (see Fig. S1). For particular values of the bias field $\vec{B}_0$, two amplifiers may be sufficient to avoid cross-excitation if the intermodulation products are far off resonance from all NV ODMR features.

Third, intermodulation products of the modulation frequencies $f_i$ may also appear in the detected PL due to insufficiently suppressed off-resonant MW cross-excitation or to NV-NV dipolar interactions. This intermodulation may occur when NV spins of a given crystallographic orientation are interrogated by two sets of modulated MWs $\nu_i$ and $\nu_j$ with different modulation frequencies $f_i$ and $f_j$. Because of the NV-center's nonlinear response to MW driving, the detected PL may be modulated not only at both $f_i$ and $f_j$, but also at sums, differences, and higher-

order products of $f_i$ and $f_j$. The strong bias field $\vec{B}_0$, along with the use of four MW amplifiers, avoids accidental near-resonant excitation by multiple MW tones in the present experiment. As shown in Fig. S4, a judicious choice of modulation frequencies $f_i$ ensures that all remaining third-order intermodulation products lie outside each channel's measurement bandwidth, and thus the present device avoids complications from intermodulation.

Fourth, we note a possible complication that should be accounted for in envisioned applications. If magnetic field signals are present at frequencies above the measurement bandwidth, these signals may be aliased into the wrong measurement channel. For example, a high-frequency field causing shifts in the $\text{NV}_\chi$ ODMR line could be detected in the band corresponding to the $\text{NV}_\kappa$ ODMR line and be misinterpreted as a low-frequency field along the $\text{NV}_\kappa$ symmetry axis. However, such spurious signals could be rejected in postprocessing by requiring that sensed signals correspond to geometrically possible field vectors. Such a requirement would eliminate, for example, signal waveforms appearing in only a single measurement channel.

## S3. MAGNETOMETER CALIBRATION AND OFF-AXIS FIELD NULLING

Because the optical table used in the present experiment is made from ferromagnetic steel, the magnetic fields detected at the diamond sensor differ from the expected fields calculated from the known coil and diamond geometry [2, 5]. For this reason, the simultaneous vector magnetometer is calibrated by conventional sequential magnetometry using the same experimental setup. Sequentially addressing the NV ODMR lines yields lock-in signal slopes $dS_i/d\Delta\nu_i$ that differ from the simultaneous measurement lock-in signal slopes by up to 1%. This difference is consistent with a $\sim$1% increase in the ODMR linewidth of the probed NV orientation when the other NV orientations are driven with near-resonant modulated MWs. The linewidth increase is observed by comparing the PL signal measured by sweeping a MW tone over one ODMR feature both with and without application of resonant MWs to ODMR features from the other NV orientations. We hypothesize that the broadening is caused by driving NV spins from other orientations out of the $m_s = 0$ state into the $m_s = \pm 1$ states, thereby increasing NV-NV dipolar interactions.

The magnetic fields from the coils oriented along the two horizontal directions $\hat{x}$ and $\hat{z}$ are observed (using both sequential and simultaneous vector magnetometry) to be distorted due to the ferromagnetic optical table, resulting in nonzero magnetic field components along the vertical $\hat{y}$ direction. The off-axis components are approximately $\sim 20\,\%$ of the total field produced by each coil. In contrast, components of $x$-coil's field along the $z$-axis and vice versa occur at the few-percent level and are attributed to error in coil alignment. Signal from the $y$-coil appearing along $\hat{x}$ and $\hat{z}$ is similarly negligible. The observed distortion of the $x$-coil and $z$-coil signals along $\hat{y}$ is consistent with numerical simulations of the coils and the ferromagnetic optical table using the Radia package in Mathematica [6, 7], up to the uncertainty of the table's relative permeability. To effectively null the off-axis fields, small currents at the frequencies $f_x = 67\,\text{Hz}$ and $f_z = 18\,\text{Hz}$ were applied to the $y$-oriented coil. The effectiveness of the field nulling was verified through standard NV vector magnetometry using sequential addressing of the NV resonances. Remaining non-idealities in the applied fields at the few-percent level, which can be seen in Fig. 4 of the main text, are attributed to imperfect off-axis field nulling and error in coil alignment.

## S4. HIGH BANDWIDTH VECTOR SENSING DEMONSTRATION

Figure S2 shows simultaneous sensing of all Cartesian components of high-frequency vector magnetic fields, achieved by operating the present device with higher modulation frequencies than employed in the main text to achieve $\approx 12.5\,\text{kHz}$ measurement bandwidth. Test magnetic fields at $1\,\text{kHz}$ and $10\,\text{kHz}$ were generated by applying sinusoidal currents to the coils aligned along $\hat{x}$ and $\hat{z}$, respectively. The magnetic field vector was reconstructed from the frequency shifts detected from three NV orientations: $\lambda$, $\chi$, and $\varphi$. Modulation frequencies $f_\lambda = 40.896\,\text{kHz}$, $f_\chi = 12.780\,\text{kHz}$, and $f_\varphi = 68.160\,\text{kHz}$ were used, with carrier frequencies and frequency deviations identical to those employed in the sensing demonstration in the main text, reported in Table I. The PL was digitized at $F_s = 204.480\,\text{kSa/s}$ and converted to ODMR line center frequency shifts via measured lock-in signal slopes: $dS_\lambda/d\Delta\nu_\lambda = 9.2\,\mu\text{V/kHz}$, $dS_\chi/d\Delta\nu_\chi = 16.6\,\mu\text{V/kHz}$, and $dS_\varphi/d\Delta\nu_\varphi = 7.0\,\mu\text{V/kHz}$. The observed reductions in signal slope are consistent with reduced ODMR contrast at higher modulation frequencies due to the finite cycling time of the NV quantum states [1, 2, 8].

Recorded PL data were digitally demodulated and band-pass filtered from 80 Hz to 12.5 kHz. The maximum sampling rate $F_s^{\max} = 204.8\,\text{kSa/s}$ of the digitizers used in the present device limited this demonstration to modulation frequencies $< F_s^{\max}/2 = 102.4\,\text{kHz}$. In addition, the modulation frequencies were chosen to divide evenly into the sampling rate to avoid aliasing effects, which limited the highest modulation frequency to $F_s/3$. Meeting these requirements for $\approx 12.5\,\text{kHz}$ measurement bandwidth resulted in several harmonics and intermodulation products of the modulation frequencies being located in the frequency encoding bands of the measurement channels. Therefore, 1-Hz-wide FFT filters were employed to remove harmonics and intermodulation products of the modulation and signal frequencies. Optimal high bandwidth sensing with this method would require use

of higher modulation frequencies (and thus higher signal sampling rate) than employed here to ensure that harmonics and intermodulation products fall outside the encoding bands of the measurement channels.

The detected ODMR line shifts were transformed into Cartesian magnetic field components via the linearized method discussed in the main text, using in place of $\mathbf{A}$ the $3\times 3$ submatrix $\mathbf{A}'$ consisting of the first three rows of $\mathbf{A}$, and using its inverse $(\mathbf{A}')^{-1}$ in place of $\mathbf{A}^{+}$. Because of the ferromagnetic optical table and $\sim 20\,\mathrm{mH}$ inductances in the magnetic field coils, pick-up of the 10 kHz signals by coils aligned along the other two axes is expected, along with interference from other metallic elements in the setup, resulting in non-negligible 10 kHz magnetic field components detected along $\hat{x}$, $\hat{y}$, and $\hat{z}$. No field-nulling currents were applied to the coils in this demonstration.

## S5. ODMR HYPERFINE FEATURES

Figure S3 displays an ODMR spectrum from the diamond sensor crystal employed in the present work at the bias field $\vec{B}_0$, for various MW drive strengths. Each of the eight main ODMR features exhibits subfeatures corresponding to splittings from the NV electric quadrupole moment and the hyperfine interaction between the NV electronic spin and the $^{14}$N nuclear spin ($I = 1$) [9]. The three principal subfeatures correspond to allowed M1 magnetic dipole transitions $\Delta m_I = 0$ [10], and the two smaller outer subfeatures (along with a third unresolved subfeature) correspond to forbidden transitions with $\Delta m_I = \pm 1$. These forbidden spin transitions have been previously observed [11] and arise from state mixing mediated by the significant off-axis components of the bias magnetic field $\vec{B}_0$. As shown in Fig. S3, the locations of these subfeatures are in good agreement with theoretical calculations of the forbidden transition frequencies [9, 10]. The relative intensity of the forbidden-transition subfeatures is observed to increase with applied MW power.

## S6. ANISOTROPIC VECTOR SENSITIVITY

For a vector magnetometer that measures field projections along multiple fixed axes in space, the response to a magnetic field's magnitude may vary with the field's direction. As a result, the device sensitivity may be anisotropic, in that higher-precision estimation of a magnetic field's magnitude may be possible when the field is oriented along certain directions relative to other directions. Consider for example a two-dimensional vector projection magnetometer with sensing axes oriented along $\hat{n}_1 = \hat{x}$ and $\hat{n}_2 = \hat{y}$. A field $\vec{B}_{\mathrm{sens}}$ will produce a different net signal on the vector magnetometer depending on the field's angular orientation. If $\vec{B}_{\mathrm{sens}}$ projects equally on $\hat{x}$ and $\hat{y}$, e.g., $\vec{B}_{\mathrm{sens}} = (B_{\mathrm{sens}}/\sqrt{2})\hat{x} + (B_{\mathrm{sens}}/\sqrt{2})\hat{y}$, then the total detected signal $S_{\mathrm{net}}$ is given by

$$\begin{aligned} S_{\mathrm{net}} &= |S_1| + |S_2| \\ &\propto |\vec{B}_{\mathrm{sens}} \cdot \hat{x}| + |\vec{B}_{\mathrm{sens}} \cdot \hat{y}| \\ &\propto B_{\mathrm{sens}}/\sqrt{2} + B_{\mathrm{sens}}/\sqrt{2} \\ &\propto B_{\mathrm{sens}}\sqrt{2}, \end{aligned} \tag{S1}$$

whereas if $\vec{B}_{\mathrm{sens}}$ is oriented along $\hat{x}$, then the total detected signal is instead only $S_{\mathrm{net}} \propto B_{\mathrm{sens}}$.

For an NV-diamond-based four-axis vector magnetometer operating in the low-field regime (where the approximation that the ODMR line shifts are proportional to the on-axis magnetic field projections is valid), the net signal is

$$S_{\mathrm{net}} \propto |\vec{B}_{\mathrm{sens}} \cdot \hat{n}_{\lambda}| + |\vec{B}_{\mathrm{sens}} \cdot \hat{n}_{\chi}| + |\vec{B}_{\mathrm{sens}} \cdot \hat{n}_{\varphi}| + |\vec{B}_{\mathrm{sens}} \cdot \hat{n}_{\kappa}|. \tag{S2}$$

Figures S5(a) and S5(b) show the expected net signal on a four-axis NV vector projection magnetometer from a unit-magnitude magnetic field as a function of field direction. In this simplified case, magnetic fields oriented along the crystal lattice vectors [100], [010], and [001], produce the largest net signal of any field orientation. We note that fields with these orientations project equally on all four NV symmetry axes. In contrast, the net signal is minimized for fields oriented along the crystal lattice vectors [110] and [$\bar{1}$10].

For an NV-diamond-based four-axis vector magnetometer operating in the general regime (where magnetic field projections both parallel and transverse to the NV symmetry axes may cause ODMR line shifts), the net signal for small $\vec{B}_{\mathrm{sens}}$ is

$$S_{\mathrm{net}} \propto |\mathbf{A}_1 \cdot \vec{B}_{\mathrm{sens}}| + |\mathbf{A}_2 \cdot \vec{B}_{\mathrm{sens}}| + |\mathbf{A}_3 \cdot \vec{B}_{\mathrm{sens}}| + |\mathbf{A}_4 \cdot \vec{B}_{\mathrm{sens}}|, \tag{S3}$$

where $\mathbf{A}_i$ is the $i^{\mathrm{th}}$ row of the linearized matrix $\mathbf{A}$, discussed in the main text. Equation S3 can be used to determine the angular dependence of the net signal from a fixed-magnitude magnetic field on the present device in the bias field $\vec{B}_0 = (3.54, 1.73, 6.95)\,\mathrm{mT}$, as depicted in Fig. S5(c). As shown in Fig. S5(d), the more generalized treatment (Eqn. S3) introduces a non-negligble shift in the anisotropy compared to that predicted by the simple projection-based treatment (Eqn. S2).

[1] C. S. Shin, C. E. Avalos, M. C. Butler, D. R. Trease, S. J. Seltzer, J. P. Mustonen, D. J. Kennedy, V. M. Acosta, D. Budker, A. Pines, and V. S. Bajaj, Journal of Applied

Physics **112**, 124519 (2012).

[2] J. F. Barry, M. J. Turner, J. M. Schloss, D. R. Glenn, Y. Song, M. D. Lukin, H. Park, and R. L. Walsworth, Proceedings of the National Academy of Sciences **113**, 14133 (2016).

[3] J. Vanier and C. Audoin, *The Quantum Physics of Atomic Frequency Standards* (A. Hilger, 1989).

[4] V. M. Acosta, E. Bauch, M. P. Ledbetter, C. Santori, K.-M. C. Fu, P. E. Barclay, R. G. Beausoleil, H. Linget, J. F. Roch, F. Treussart, S. Chemerisov, W. Gawlik, and D. Budker, Phys. Rev. B **80**, 115202 (2009).

[5] G. Chatzidrosos, A. Wickenbrock, L. Bougas, N. Leefer, T. Wu, K. Jensen, Y. Dumeige, and D. Budker, Phys. Rev. Applied **8**, 044019 (2017).

[6] P. Elleaume, O. Chubar, and J. Chavanne, in *Proceedings of the 1997 Particle Accelerator Conference*, Vol. 3 (1997) pp. 3509–3511.

[7] O. Chubar, P. Elleaume, and J. Chavanne, Journal of Synchrotron Radiation **5**, 481 (1998).

[8] K. Jensen, N. Leefer, A. Jarmola, Y. Dumeige, V. M. Acosta, P. Kehayias, B. Patton, and D. Budker, Phys. Rev. Lett. **112**, 160802 (2014).

[9] M. W. Doherty, F. Dolde, H. Fedder, F. Jelezko, J. Wrachtrup, N. B. Manson, and L. C. L. Hollenberg, Phys. Rev. B **85**, 205203 (2012).

[10] V. M. Acosta, *Optical magnetometry with nitrogen-vacancy centers in diamond*, Ph.D. thesis, University of California, Berkeley (2011).

[11] S. Felton, A. M. Edmonds, M. E. Newton, P. M. Martineau, D. Fisher, D. J. Twitchen, and J. M. Baker, Phys. Rev. B **79**, 075203 (2009).

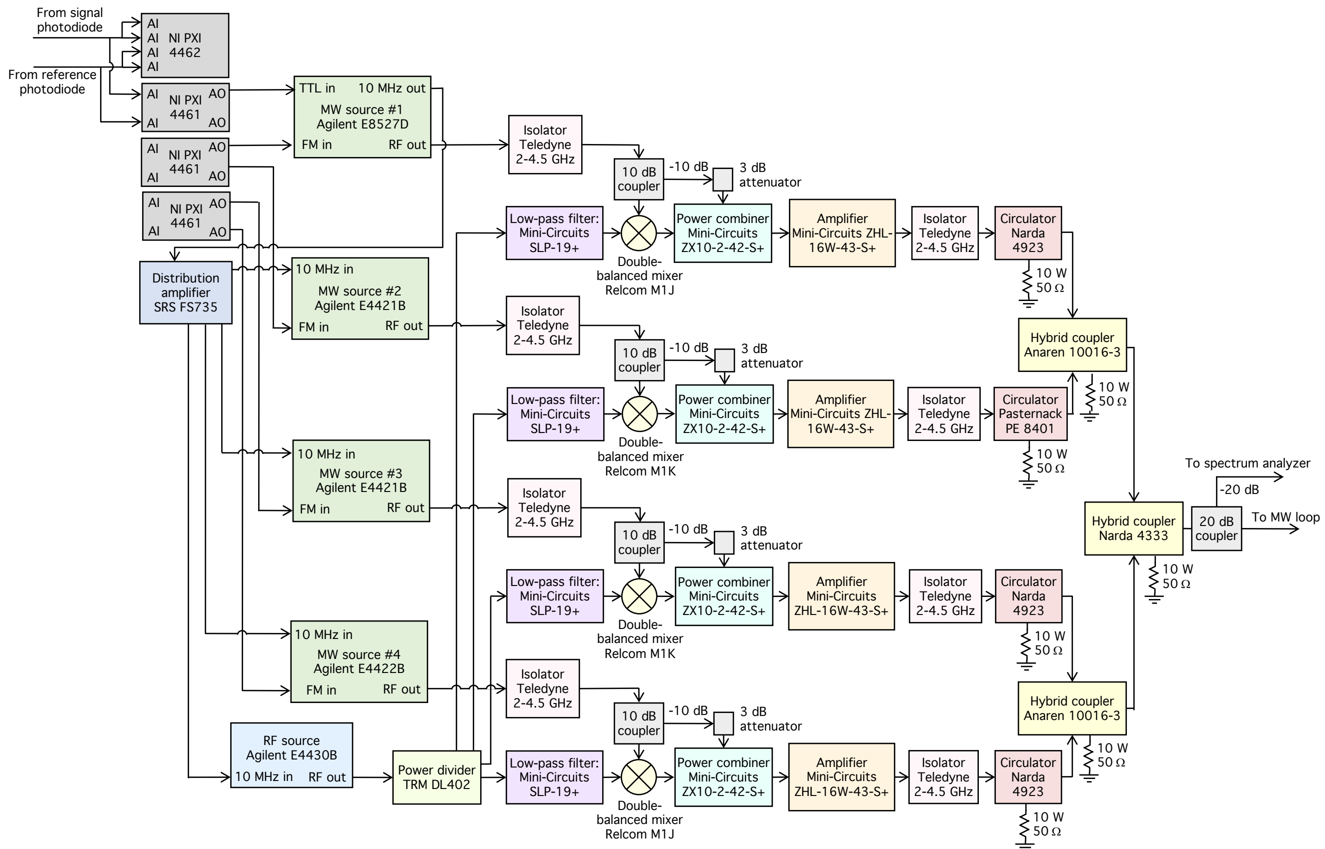


FIG. S1. Electronic equipment used to generate MW tones to drive four NV orientations in the simultaneous vector magnetometer. Analog inputs and outputs are abbreviated AI and AO.

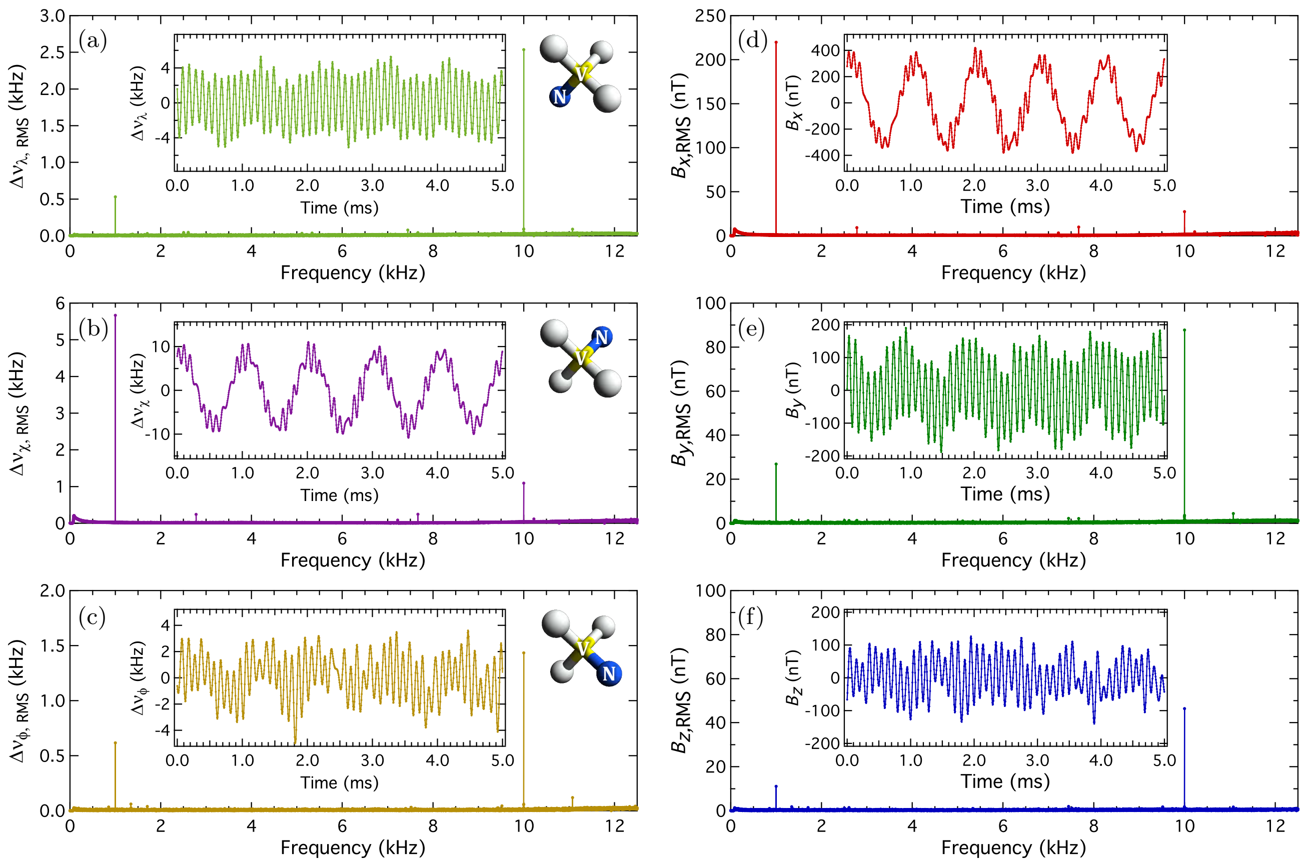


FIG. S2. Simultaneous vector magnetic sensing of high-frequency fields with ≈12.5 kHz measurement bandwidth. Sinusoidal magnetic fields were applied at 1 kHz and 10 kHz. a-c) Frequency shifts of ODMR line centers detected from three NV orientations: $\lambda$, $\chi$, and $\varphi$. d-f) Cartesian field components reconstructed from detected frequency shifts. Modulation frequencies $f_\lambda = 40.896$ kHz, $f_\chi = 12.780$ kHz, and $f_\varphi = 68.160$ kHz were employed, and PL was sampled at $F_s = 204.480$ kSa/s. Several notch-stop filters removed cross-talk from harmonics and intermodulation products of the modulation and signal frequencies. As discussed in Section S4, achieving cross-talk-free sensing (see main text Figs. 3 and 4) with ≈12.5 kHz measurement bandwidth requires modest technical upgrades to the device.

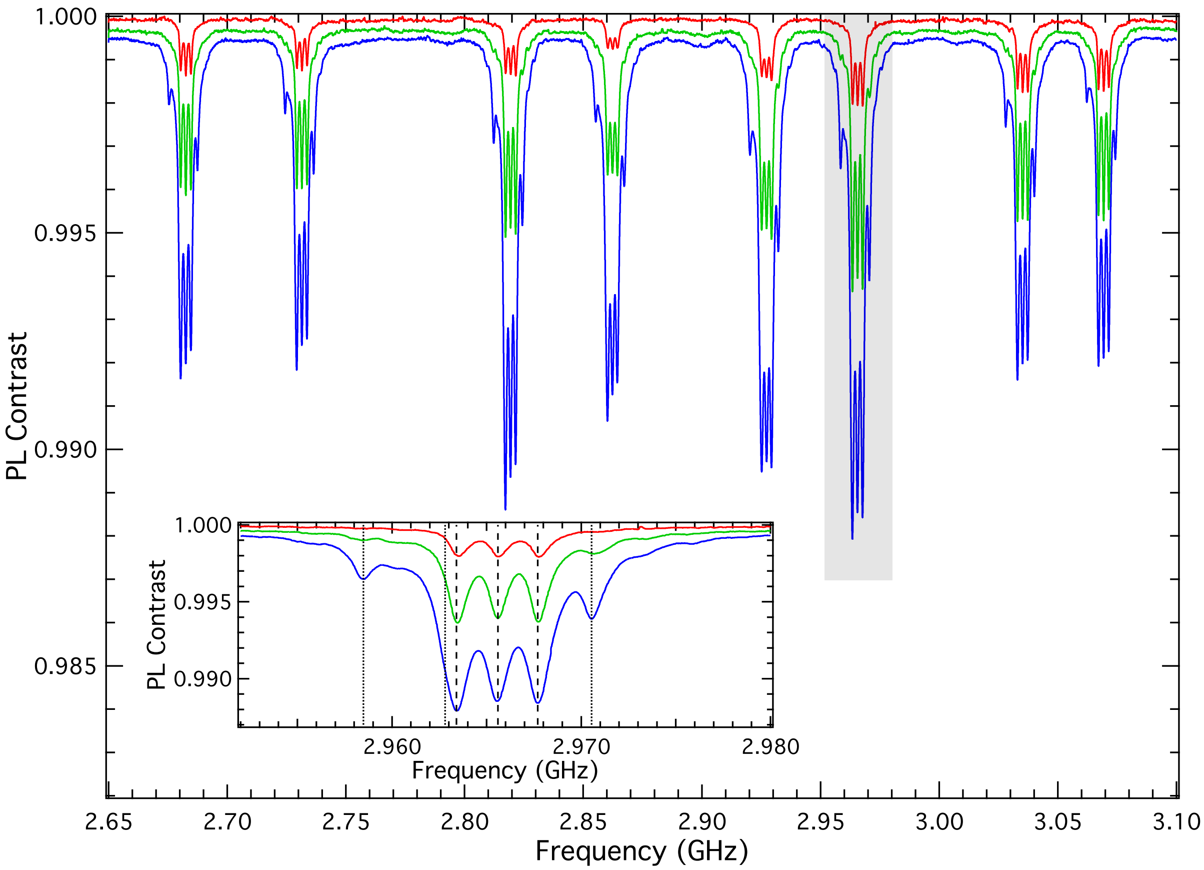


FIG. S3. ODMR spectrum of an NV ensemble in applied bias field $|\vec{B}_0| = 7.99\,\text{mT}$, $\vec{B}_0 = (3.54, 1.73, 6.95)\,\text{mT}$ for various MW drive strengths. The blue (highest contrast) trace depicts the spectrum with MW power typical of operating conditions, while the green (middle) and red (lowest contrast) traces depict the same spectrum with MW power reduced by 12 and 24 dB, respectively. The subfeatures within the eight main ODMR features correspond to splittings associated with the NV center's electric quadrupole moment and the hyperfine interaction between the NV electronic spin and $^{14}$N nuclear spin ($I = 1$) [9]. The three principal subfeatures correspond to allowed M1 magnetic dipole transitions with $\Delta m_I = 0$, and the two smaller subfeatures correspond to forbidden transitions with $\Delta m_I = \pm 1$, which appear due to state mixing mediated by the significant off-axis magnetic field [11] and are more pronounced for stronger MW drive. Inset shows the ODMR feature enclosed in the gray box. Dashed lines mark the allowed hyperfine transitions [9, 10]; dotted lines mark the frequencies associated with forbidden hyperfine transitions between states of different $m_I$ [10, 11]. Traces are slightly offset for clarity in both main figure and inset.

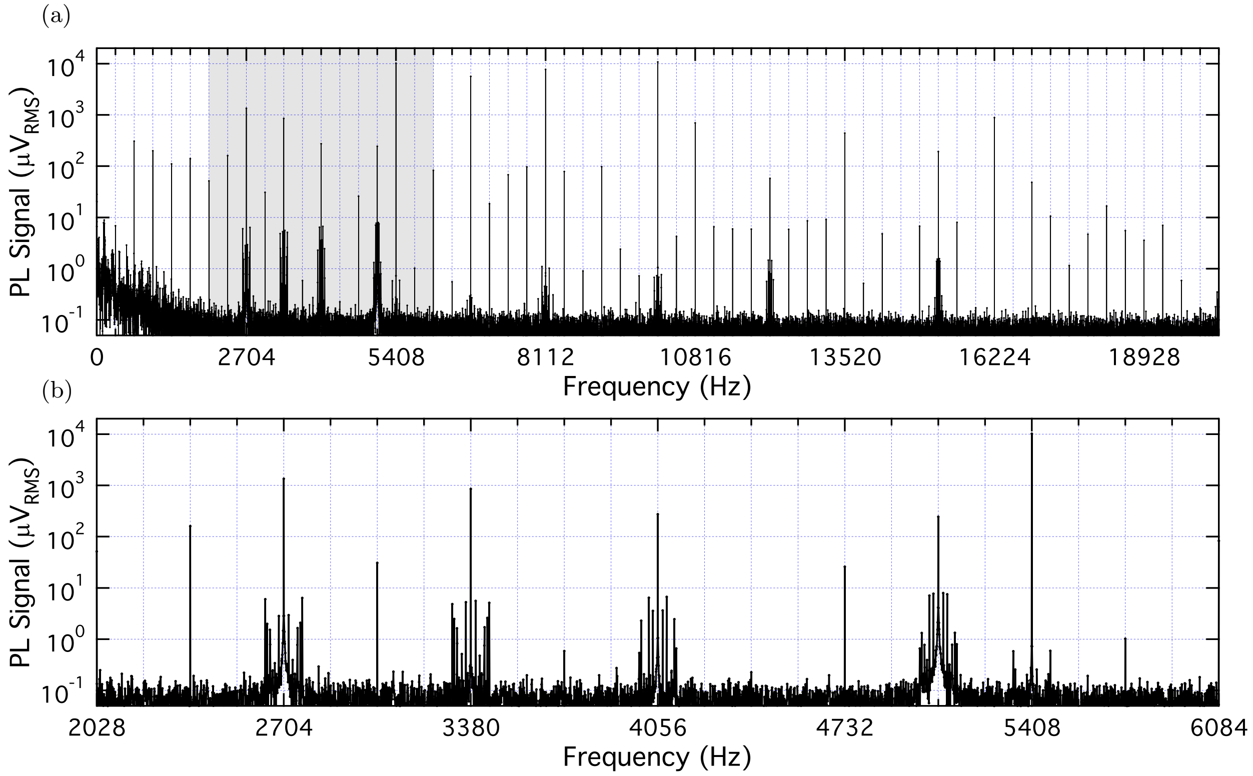


FIG. S4. Spectral density from vector magnetometry demonstration described in the main text and displayed in Figs. 3 and 4 after laser noise cancellation. In (a), low-frequency noise is apparent, revealing the utility of modulated ODMR to approach shot-noise-limited magnetometry. Harmonics and intermodulation products of the modulation frequencies $f_i$ are also visible. Magnetic signals encoded around the harmonics are reduced by $\sim 10\times$ compared to signals around the fundamental $f_i$, and signals around the intermodulation products are below the noise floor. (b) Zoomed-in plot of gray box in (a). Magnetic signals encoded around the modulation frequencies $f_i$ are visible, along with intermodulation products of $f_i$ and the harmonic at $2f_\chi = 5408\,\mathrm{Hz}$.

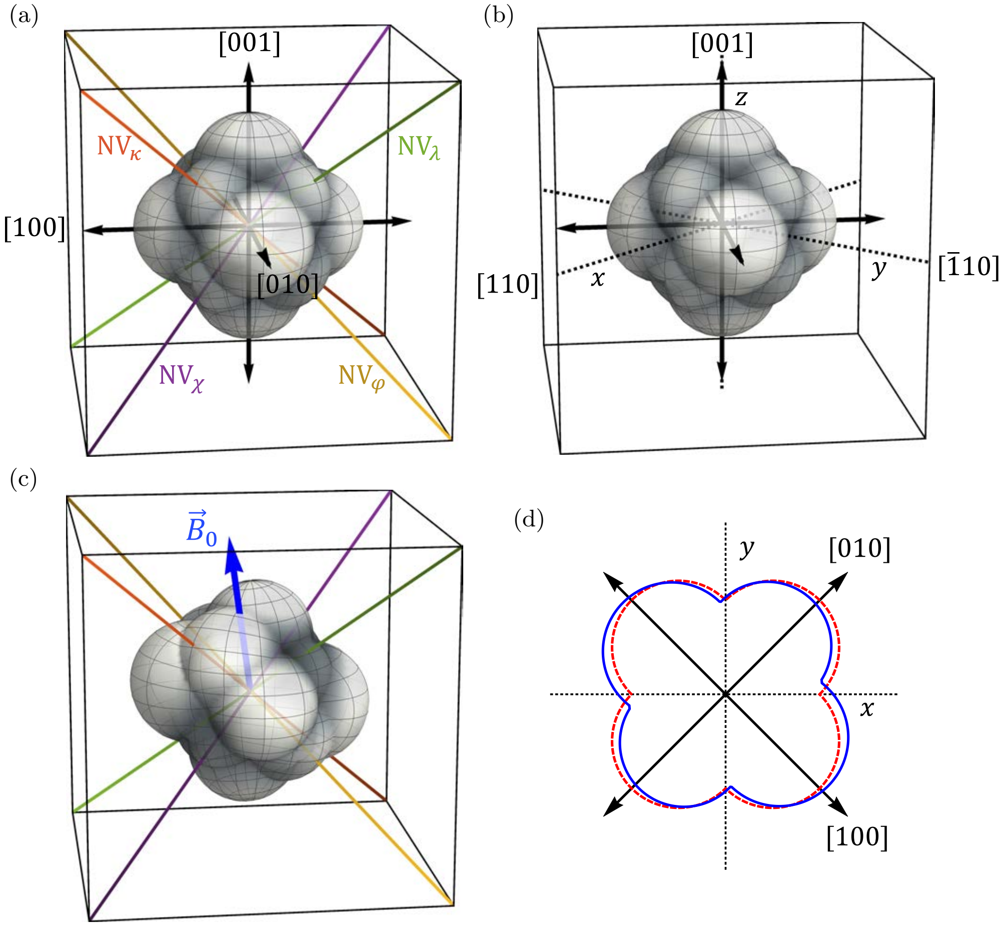


FIG. S5. Anisotropy of vector magnetometer response. (a) Net signal on a four-axis projection-based NV-diamond magnetometer versus direction for a fixed-magnitude magnetic field $\vec{B}_{\text{sens}}$. The response is largest for magnetic fields oriented parallel or antiparallel to the diamond crystal lattice vectors ([100], [010], [001]). (b) Same as (a) but with lab-frame $x$-, $y$-, and $z$-axes. Net signal is minimized for magnetic fields along $\hat{x}$ and $\hat{y}$ ([110] and [$\bar{1}$10]). (c) Net signal on the present NV-diamond vector magnetometer in the bias field $\vec{B}_0 = (3.54, 1.73, 6.95)\,\text{mT}$, including contributions from field components both parallel and transverse to the NV symmetry axes. A slight shift of the signal anisotropy compared to (a) is apparent. (d) Slices of the surface plots in (a) and (c) for $z=0$. Red dashed (- -) and blue solid (–) curves respectively mark the net signal from the simplified projection-based magnetometer, and from the present magnetometer.
